# Supplementary material for: Vanishing Hall Conductance in the Phase Glass Bose Metal at Zero Temperature
Source: arXiv:1708.09016 source file (2017-08-29)
Supplement: Supplementary file 1 [file Supplementalbm.pdf]

# Supplemental Material for "Vanishing Hall Conductance in the Phase Glass Bose Metal at Zero Temperature"

Julian May-Mann and Philip W. Phillips
*Department of Physics, University of Illinois at Urbana-Champaign, Urbana, Illinois, USA*

## APPENDIX

Here we will briefly show that the contribution to the Hall conductance is 0 at linear order in $U$ if there is particle hole symmetry. Furthermore, we will also explicitly show that the vertex diagram, Fig 1 (b) does not contribute independently from the actual form of the Gaussian propagator. The linear order corrections to the Hall conductance are shown in Fig 1. It has been shown that this loop correction can be expressed as a correction to the mass term of the free energy [1],

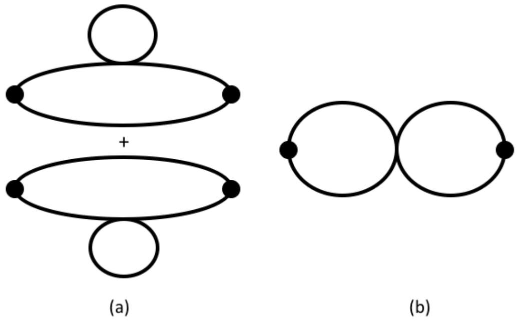


FIG. 1. The two diagrams that contribute to the Hall Conductance in the presence of a broken particle-hole symmetry (a) the loop correction that which will be expressed as a rescaling of the mass and (b) the vertex correction.

$$\delta m^2 = \frac{UTm_H^2}{4\imath} \sum_{\omega_n, l} [G_0(l,\omega_n) + \beta\delta_{\omega_n,0} q G_0^2(l,\omega_n)]. \quad (1)$$

Since this does affect the particle hole symmetry of the propagator, the result from Gaussian level shows that this contribution is zero.

We now will explicitly calculate the contribution from diagram 1 (b). In full, the contribution to the Hall conductance is

$$\begin{aligned}\sigma_H(i\omega_\nu) = {} & \frac{i(e^* m_H)^2}{2\omega_\nu \hbar\beta} \sum_{\substack{a,b,c,l,l',p_y,p'_y,\\ p''_y,\omega_n,\omega'_n,\omega''_n}} \int dz \int d\tau e^{i\omega_\nu \tau} \sqrt{(l+1)(l'+1)} \\ & \times \langle (C^a_{l,p_y}(\omega_n) C^{a*}_{l+1,p_y}(\omega_n) + C^a_{l+1,p_y}(\omega_n) C^{a*}_{l,p_y}(\omega_n)) \\ & \times (C^b_{l',p'_y}(\omega'_n) C^{b*}_{l'+1,p''_y}(\omega''_n) - C^b_{l'+1,p'_y}(\omega'_n) C^{b*}_{l',p''_y}(\omega''_n)) \\ & \times \frac{U}{2} \sum_{l_i,\omega_j,p_{yk}} C^c_{l_1,p_{y1}}(\omega_1) C^{*c}_{l_2,p_{y2}}(\omega_2) C^c_{l_3,p_{y3}}(\omega_3) C^{*c}_{l_4,p_{y4}}(\omega_4) \rangle \\ & \times \phi_{l_1}(z - \frac{\hbar p_{y1}}{e^* B}) \phi_{l_2}(z - \frac{\hbar p_{y2}}{e^* B}) \phi_{l_3}(z - \frac{\hbar p_{y3}}{e^* B}) \phi_{l_4}(z - \frac{\hbar p_{y4}}{e^* B}) \\ & \times \delta_{\Sigma\omega_j,0} \delta_{\Sigma p_{yk},0}.\end{aligned} \quad (2)$$

We will now fix $l$ and $l'$ and focus on the contribution of

$$\begin{aligned}B(l_i) = {} & \sum_{\substack{a,b,p_y,p'_y,\\ p''_y,\omega_n,\omega'_n,\omega''_n}} \int dz \langle ((C^a_{l_1,p_y}(\omega_n) C^{a*}_{l_2,p_y}(\omega_n) (C^b_{l_3,p'_y}(\omega'_n) C^{b*}_{l_4,p''_y}(\omega''_n) \\ & \times \frac{U}{2} \sum_{l'_i,\omega_j,p_{yk}} C^a_{l_1,p_{y1}}(\omega_1) C^{*a}_{l_2,p_{y2}}(\omega_2) C^a_{l_3,p_{y3}}(\omega_3) C^{*a}_{l_4,p_{y4}}(\omega_4) \rangle \\ & \times \phi_{l'_1}(z - \frac{\hbar p_{y1}}{e^* B}) \phi_{l'_2}(z - \frac{\hbar p_{y2}}{e^* B}) \phi_{l'_3}(z - \frac{\hbar p_{y3}}{e^* B}) \phi_{l'_4}(z - \frac{\hbar p_{y4}}{e^* B}) \\ & \times \delta_{\Sigma\omega_j,0} \delta_{\Sigma p_{yk},0}.\end{aligned} \quad (3)$$

Eq. 2 is then simply

$$\begin{aligned}\sigma_H(i\omega_\nu) = {} & \frac{i(e^* m_H)^2}{2\omega_\nu \hbar\beta} \sum_{l,l'} \int dz \int d\tau e^{i\omega_\nu \tau} \sqrt{(l+1)(l'+1)} \\ & \times [B(l,l+1,l',l'+1) + B(l+1,l,l',l'+1) \\ & - B(l,l+1,l'+1,l') - B(l+1,l,l'+1,l')].\end{aligned} \quad (4)$$

Returning to Eq. 3, and using Wick's theorem and that $\langle C^a_{l,p_y}(\omega) C^{*b}_{l',p'_y}(\omega') \rangle = G^{ab}(l,p_y,\omega) \delta_{l,l'} \delta_{p_y,p'_y} \delta_{\omega,\omega'}$, we then have

$$B(l_i) = 2U \sum_{\substack{a,b,p_y,p'_y,\\ p''_y,\omega_n,\omega'_n,\omega''_n}} \int dz (G^{ac}(l_1, p_y \omega_n) G^{ac}(l_2, p_y, \omega_n) \\ \times G^{bc}(l_3, p'_y, \omega'_n) G^{bc}(l_4, p''_y \omega''_n) \\ \times \phi_{l_1}(z - \frac{\hbar p_y}{e^* B}) \phi_{l_2}(z - \frac{\hbar p_y}{e^* B}) \phi_{l_3}(z - \frac{\hbar p_{y'}}{e^* B}) \phi_{l_4}(z - \frac{\hbar p_{y''}}{e^* B}) \\ \times \delta_{\omega'_n - \omega''_n, 0} \delta_{p'_y - p''_y, 0}. \quad (5)$$

Summing over $p_y$, we find that there is the term in the propagator that is independent of $p_y$ (see the expression defining the full propagator in the text). So the only $p_y$ dependence is from the $\phi$ functions. Therefore,

$$B(l_i) \propto \sum_{p_y} \phi_{l_1}(z - \frac{\hbar p_y}{e^* B}) \phi_{l_2}(z - \frac{\hbar p_y}{e^* B}) = \delta_{l_1, l_2}, \quad (6)$$

where we have used the orthonormality of the eigenfunctions of the harmonic oscillator. Plugging Eq. (6) into Eq. (4) we see that $\lim_{\omega_\nu \to 0} \sigma_H(\omega_\nu) = 0$. This is true for any propagator, provided that it is independent of $p_y$. Since this is true of the phase glass, both with and without particle hole symmetry, we conclude that Fig 1 (b) does not contribute in either case.

[1] J. Wu and P. Phillips, Phys. Rev. B **73**, 214507 (2006), cond-mat/0512432.
